# Supplementary material for: Active Property Testing
Source: arXiv:1111.0897 source file (2012-04-17)
Supplement: Supplementary file 2 [file appendix-general.tex]

Recall that we defined the \emph{local characterization} of properties as follows:

\newtheorem*{deflocalchar}{Definition~\ref{def:localchar}}
\begin{deflocalchar} 
Fix $\delta > 0$ and $\eps' > 0$.
The property $\calP$ of functions $f : D \to R$ is \emph{($\delta, \eps'$)-locally characterized}
 by the property $\calP'$ if there exist
a metric $\rho : D \times D \to \reals$ and a radius $r > 0$ such that for a 
 domain $D' \subseteq D$ obtained by choosing
$x \in D$ uniformly at random and setting $D' = \{y : \rho(x,y) \le r\}$, the following two conditions
are satisfied:
\begin{enumerate}
\item When $f \in \calP$, then $\Pr_{D'}[ f|_{D'} \in \calP' ] \ge \frac12 + \delta$, and
\item When $f$ is $\eps$-far from $\calP$, then $\Pr_{D'}[ f|_{D'} \mbox{ is $\eps'$-far from } \calP'] \ge \frac12 + \delta$.
\end{enumerate}
\end{deflocalchar}

We refer to the radius $r$ in the definition above as the 
\emph{local characterization radius} of $\calP$ by $\calP'$.  
Our general reduction is the following lemma, which shows that
if a property $\calP$ is locally characterized by some property $\calP'$
which can be efficiently tested in the passive model, then $\calP$ can
be efficiently tested in the active model:

\begin{lemma}
\label{lem:general}
Let $\calP$ be $(\delta,\eps')$-locally characterized by a property $\calP'$ which can
be $\eps'$-tested in the passive model with $s$ samples.  If the local characterization
radius $r$ of $\calP$ by $\calP'$ satisfies 
$$
\Pr_{x,y \sim \calD}[ \rho(x,y) \le r] \ge \gamma,
$$
then $\calP$ can
be $\eps$-tested in the active model over the distribution $\calD$ with $O(s \log \frac1\delta)$ queries from 
$O(s/\gamma \log\frac1\delta)$ unlabeled examples.
\end{lemma}

\begin{proof}
The tester for $\calP$ is a generalization of the union of interval tester and the 
cluster assumption tester.  Specifically, we set the tester to do the following:
\begin{enumerate}
\item Repeat $t = O(\log \frac1\delta)$ times:
\begin{enumerate}
\item[1.1] Draw $x$ uniformly at random from $D$.
\item[1.2] Set $D' = \{y \in D : \rho(x,y) \le r\}$.
\item[1.3] Draw at most $O(s/\gamma)$ samples from $D$ until we obtain $y^1,\ldots,y^{s-1} \in D'$.
If we fail, return to Step 1.1.
\item[1.4] Use $\calP'$'s tester and the points $x,y^1,\ldots,y^{s-1}$ to test
whether $f|_{D'} \in \calP$.
\end{enumerate}
\item Accept iff at least $\frac12$ of the tests in Step 1.4 accept.
\end{enumerate}

The tester makes $s$ queries at each iteration of the steps 1.1 and 1.4, so it has the desired
query complexity.  The condition on the probability that $\rho(x,y) \le r$ guarantees that
Step 1.3 will fail rarely, so we obtain the desired complexity on the number of unlabeled 
examples as well.  

To complete the proof, we want to establish the correctness of the tester. This follows
from a Chernoff bound argument: the algorithm computes an estimate of 
$\Pr_{D'}[ f|_{D'} \in \calP']$, when $t = c \log \frac1\delta$ for some large enough constant $c$, 
the probability that this estimate differs from its true value by more than $\delta$ -- and thus
the probability that the tester for $\calP$ errs -- is at most $\frac13$.
\end{proof}

In light of Lemma~\ref{lem:general}, the problem of designing a query-efficient
active tester for a property $\calP$ can be reduced to the problem of showing
that this property can be locally characterized by a particularly simple (and efficiently
testable) property $\calP'$.  In particular, we can obtain an alternative proof of the active
testing bound in Theorem~\ref{thm:ui-act} in this way:

\begin{lemma}
The property of being a union of $d$ intervals is ($?$,$?$)-locally characterized by
the \emph{constant} property (i.e. the property containing only the two constant functions
$f(x) = 0$ and $f(x) = 1$).
\end{lemma}

\begin{proof}
Define the local characterization radius to be $r = \frac{\eps^2}{32d}$.  When $f$ is a union
of $d$ intervals, the probability that $f|_{D'}$ is constant over a uniformly chosen interval
$D'$ of length $2r$ is at least $1 - \frac{\eps^2}8$.
\end{proof}
